# Supplementary material for: Team Enigma at ArgMining-EMNLP 2021: Leveraging Pre-trained Language Models for Key Point Matching
Source: arXiv:2110.12370 source file (2021-10-24)
Supplement: Supplementary file 1 [file appendix.tex]

\setcounter{section}{9}

\vspace{+1cm}
\section*{\centering{Appendix : Supplementary Material}} 
\label{sec:appendix}
\vspace{-0.0cm}

\subsection{Appendix A}

The Tables \ref{tab: appendix dependency features} and \ref{tab:appendix POS features} show the list of top ten frequently occurring dependency feature tags and POS (Part Of Speech) tags along with their brief explanations.

\begin{table}[!htb]
\centering
%\resizebox{\columnwidth}{!}{
\begin{tabular}{cc}
\hline
\multicolumn{1}{l}{\textbf{Dependency Tag}} & \multicolumn{1}{l}{\textbf{Short Explanation}} \\
\hline
aux      & Auxiliary              \\
nsubj    & Nominal subject        \\
amod     & Adjectival modifier    \\
dobj     & Direct object          \\
prep     & Prepositional modifier \\
pobj     & Object of preposition  \\
\small{ROOT}     & Root                   \\
compound & Compound               \\
conj     & Conjunct               \\
ccomp    & Clausal complement    \\
\hline
\end{tabular}
%}
\caption{Top ten frequent dependency features}
\label{tab: appendix dependency features}
\end{table}

\begin{table}[!htb]
\centering
%\resizebox{\columnwidth}{!}{
\begin{tabular}{cc}
\hline
\textbf{POS Tag} & \textbf{Short Explanation} \\

\hline
\small{VERB}             & Verb                       \\
\small{NOUN}             & Noun                       \\
\small{AUX}              & Auxiliary                  \\
\small{ADP}              & Adposition                 \\
\small{ADJ}              & Adjective                  \\
\small{PROPN}            & Proper noun                \\
\small{SCONJ}            & Subordinating conjunction  \\
\small{ADV}            & Adverb                     \\
\small{PRON}             & Pronoun                    \\
\small{DET}              & Determiner          \\
\hline
\end{tabular}
%}
\caption{Top ten frequent POS features}
\label{tab:appendix POS features}
\end{table}

\newpage
\subsection{Appendix B}

Tables \ref{tab:appendix dependency table}, \ref{tab:appendix pos table} and \ref{tab:appendix tfidf table} report complete results\footnote{All the reported results are according to the default evaluation method for \emph{mAP} strict and \emph{mAP} relaxed scores (explained in section 5 of main paper)} of the transformer models with additional feature vectors, whose best results were reported in the Results and Discussion section of the paper.

\begin{table}[!htb]
\centering
\resizebox{\columnwidth}{!}{\begin{tabular}{cccc}
\hline
\textbf{Model} &
  \textbf{\begin{tabular}[c]{@{}l@{}}Feature \\ Type\end{tabular}} &
  \textbf{\begin{tabular}[c]{@{}l@{}}mAP \\ Strict\end{tabular}} &
  \textbf{\begin{tabular}[c]{@{}l@{}}mAP \\ Relaxed\end{tabular}} \\
\hline
BERT-large    & Dep\tablefootnote{Encoded dependency features} & 0.764 $\pm$ 0.035          & 0.901 $\pm$ 0.017          \\
RoBERTa-large & Dep & 0.802 $\pm$ 0.028          & 0.952 $\pm$ 0.021          \\
BART-large    & Dep & \textbf{0.868 $\pm$ 0.023} & \textbf{0.977 $\pm$ 0.015} \\
DeBERTa-large & Dep & 0.851 $\pm$ 0.029          & 0.957 $\pm$ 0.018       \\
\hline
\end{tabular}}
\caption{Results with dependency features}
\label{tab:appendix dependency table}
\end{table}

%\vspace{-0.5cm}

\begin{table}[htb!]
\centering
\resizebox{\columnwidth}{!}{\begin{tabular}{cccc}
\hline
\textbf{Model} &
  \textbf{\begin{tabular}[c]{@{}l@{}}Feature \\ Type\end{tabular}} &
  \textbf{\begin{tabular}[c]{@{}l@{}}mAP \\ Strict\end{tabular}} &
  \textbf{\begin{tabular}[c]{@{}l@{}}mAP \\ Relaxed\end{tabular}} \\
\hline
BERT-large    & POS\tablefootnote{Encoded POS features} & 0.808 $\pm$ 0.012          & 0.942 $\pm$0.012           \\
RoBERTa-large & POS & 0.859 $\pm$ 0.047          & 0.964 $\pm$0.002           \\
BART-large    & POS & \textbf{0.906 $\pm$ 0.011} & \textbf{0.987 $\pm$ 0.005} \\
DeBERTa-large & POS & 0.880 $\pm$ 0.040          & 0.968 $\pm$ 0.012     \\     
\hline
\end{tabular}}
\caption{Results with parts of speech features}
\label{tab:appendix pos table}
\end{table}

\begin{table}[htb!]
\centering
\resizebox{\columnwidth}{!}{\begin{tabular}{cccc}
\hline
\textbf{Model} &
  \textbf{\begin{tabular}[c]{@{}l@{}}Feature \\ Type\end{tabular}} &
  \textbf{\begin{tabular}[c]{@{}l@{}}mAP \\ Strict\end{tabular}} &
  \textbf{\begin{tabular}[c]{@{}l@{}}mAP \\ Relaxed\end{tabular}} \\
\hline
BERT-large    & Tf-idf & 0.830 $\pm$ 0.023          & 0.937 $\pm$ 0.018          \\
RoBERTa-large & Tf-idf & 0.870 $\pm$ 0.041         & 0.967 $\pm$ 0.013          \\
BART-large    & Tf-idf & 0.880 $\pm$ 0.029         & 0.969 $\pm$ 0.027          \\
DeBERTa-large & Tf-idf & \textbf{0.911 $\pm$ 0.005} & \textbf{0.987 $\pm$ 0.008} \\
\hline
\end{tabular}}
\caption{Results with tf-idf features}
\label{tab:appendix tfidf table}
\end{table}

%\vspace{-0.8cm}
\newpage
\subsection{Appendix C}

Table \ref{tab:appendix big table} reports the complete results\footnote{All the reported results are according to the default evaluation method for \emph{mAP} strict and \emph{mAP} relaxed scores (explained in section 5 of main paper)} of transformer models pre-trained on the additional datasets with each of the additional feature and further fine tuned on the main shared task dataset with the same type of additional feature. 

Some of the results which are marked with a dashed line could not be reported due to resource constraints.

\begin{table}[H]
\centering
\resizebox{\columnwidth}{!}{
\begin{tabular}{ccccc}
\hline
\textbf{Model} &
  \textbf{\begin{tabular}[c]{@{}c@{}}Additional \\ Dataset\end{tabular}} &
  \textbf{\begin{tabular}[c]{@{}c@{}}Feature\\  type\end{tabular}} &
  \textbf{\begin{tabular}[c]{@{}c@{}}mAP \\ Strict\end{tabular}} &
  \textbf{\begin{tabular}[c]{@{}c@{}}mAP \\ Relaxed\end{tabular}} \\
  \hline
BART-large    & STS         & POS    & 0.904 $\pm$ 0.031          & 0.985 $\pm$ 0.015          \\
DeBERTa-large & STS         & POS    & 0.877 $\pm$ 0.017          & 0.978 $\pm$ 0.011          \\
BART-large    & STS         & Dep    & 0.899 $\pm$ 0.029          & 0.984 $\pm$ 0.014          \\
DeBERTa-large & STS         & Dep    & 0.874 $\pm$ 0.042          & 0.936 $\pm$ 0.073          \\
BART-large    & STS         & Tf-idf & 0.910 $\pm$ 0.008          & 0.985 $\pm$ 0.003          \\
DeBERTa-large & STS         & Tf-idf & 0.903 $\pm$ 0.017          & 0.980 $\pm$ 0.013          \\
BART-large    & IBM Args30k & POS    & 0.912 $\pm$ 0.018          & 0.984 $\pm$ 0.002          \\
DeBERTa-large & IBM Args30k & POS    & --\tablefootnote{Due to resource constraints, we could not report values of these experimental settings}                  & --                   \\
BART-large    & IBM Args30k & Dep    & 0.890 $\pm$ 0.007          & 0.978 $\pm$ 0.006          \\
DeBERTa-large & IBM Args30k & Dep    & --                   & --                   \\
BART-large    & IBM Args30k & Tf-idf & \textbf{0.919 $\pm$ 0.007} & \textbf{0.986 $\pm$ 0.002} \\
DeBERTa-large & IBM Args30k & Tf-idf & --                   & --                   \\
\hline
\end{tabular}}
\caption{Results with pretraining on additional datasets with additional features}
\label{tab:appendix big table}
\end{table}
